# Supplementary material for: Microstructural Studies Using Generative Adversarial Network (GAN): a Case Study
Source: arXiv:2506.05860 ancillary file (2025-06-06)
Supplement: Supplementary file 1 [file supplementary_added.pdf]

# Supporting Information
# Scope of Generative Artificial Intelligence in Microstructural Studies: a Case Study

Owais Ahmad,[1] Vishal Panwar,[1] Kaushik Das,[2]
Rajdip Mukherjee,[1,*] and Somnath Bhowmick[1,†]

[1]*Department of Materials Science and Engineering,*
*Indian Institute of Technology Kanpur, Kanpur 208016, India*
[2]*Department of Metallurgy and Materials Engineering,*
*Indian Institute of Engineering Science and Technology,*
*West Bengal, Shibpur, Howrah, 711103, India*

(Dated: May 2, 2025)

## S1. PHASE-FIELD MODEL AND NUMERICAL IMPLEMENTATION

Phase transformations in materials manifest through the motion of interfaces separating two phases. During the process, one phase grows locally at the expense of the other. Modeling the motion of atomistically sharp interfaces requires explicit interface location tracking as a function of time. This process is not computationally feasible while modeling realistic phase distributions and topologies. The phase-field method deals with this difficulty by considering a diffuse interface separating the two phases. First, one assigns certain values to the phase field variables $(\phi_1, \phi_2, \cdots, \phi_N)$ within the simulation domain, indicating the presence of different equilibrium phases at those locations. The interfaces between the equilibrium phases are denoted by smooth variations of the phase fields bounded by the values given for the equilibrium phases on both sides. The temporal evolution of the phase fields captures the migration of the diffuse interface, and the resulting transformation accurately. The phase fields can be defined for either conserved (e.g., density, composition) or non-conserved (e.g., grain order parameters) quantities.

For the conserved phase-field variables (e.g., composition, density), one has to solve the Cahn-Hilliard equation[1,2] for simulating diffusion-controlled transformations. Here, we describe the numerical implementation using the semi-implicit Fourier transform method[3] to solve the fourth-order non-linear partial differential equation. Evaluating the Fourier transform of both sides of Eq. 3 (main article), we get,

$$\frac{\partial \widetilde{c(\mathbf{k})}}{\partial t} = -M[k^2 \widetilde{g_c(\mathbf{k})} + 2\kappa k^4 \widetilde{c(\mathbf{k})}]. \tag{1}$$

The overhead tildes denote fields in the Fourier space, as functions of the Fourier space vectors, denoted by $\mathbf{k}$. The magnitude of the Fourier space vectors is given by, $k = \sqrt{\sum_{i=1}^{i=d} k_i^2}$, $d$ being the number of dimensions. Note that, $g(c)$ is a non-linear function of $c$ and no simple expression exists relating the Fourier transform of $c$ to the Fourier transform of $g(c)$. Thus, we first evaluate $g(c)$ in the real space at the current instant of time $(t)$. Then, we compute its Fourier transform to obtain $\widetilde{g_c(\mathbf{k})}$, while all the other terms in Eq. 1 are evaluated at the future instant of time $t + \Delta t$. The "semi-implicit" time integration is given by[3],

$$\frac{\widetilde{c}(\mathbf{k}, t + \Delta t) - \widetilde{c}(\mathbf{k}, t)}{\Delta t} = -M[k^2 \widetilde{g_c}(\mathbf{k}, t) + 2\kappa k^4 \widetilde{c}(\mathbf{k}, t + \Delta t)], \tag{2}$$

which can be re-arranged to obtain,

$$\widetilde{c}(\mathbf{k}, t + \Delta t) = \frac{\widetilde{c}(\mathbf{k}, t) - M\Delta t k^2 \widetilde{g}_c(\mathbf{k}, t)}{1 + 2M\Delta t \kappa k^4}. \tag{3}$$

As the time integration is performed in the Fourier space, one has to revert to the real space to construct the function $g(c)$ at every timestep. This process is done by evaluating an inverse-Fourier transform of the composition fields $\widetilde{c}(\mathbf{k})$. The numerical algorithm can be summarized as,

1. Assign the initial composition field $c(\mathbf{r}, t)$ at $t = 0$,
2. Compute the function $g(c)$,
3. Evaluate the Fourier transform of $c(\mathbf{r}, t)$ and $g(c)$,
4. Time integrate in the Fourier space to obtain $\widetilde{c}(\mathbf{k}, t + \Delta t)$,
5. Compute an inverse Fourier transform to obtain the composition fields at the next instant of time $c(\mathbf{r}, t + \Delta t)$,
6. Repeat steps (2), (3), (4), and (5) to go forward in time.

The simulation box size is $256 \times 256$ grids. The scaled, non-dimensional phase-field parameters are $W = 1, \kappa = 1, M = 1$. The discretization size in space and time are $\Delta x = 1.0$, and $\Delta t = 1.0$, respectively.

## S2. VIRTUAL MECHANICAL TESTING

### A. Material Property

To do a compression test over microstructure with a composite system hypothesis, one has to provide isotropic elastic properties and plastic deformation true stress-strain data for each phase. We assume the matrix phase to be pure iron, and the precipitate phase is pure chromium. The elastoplastic properties of single crystal iron and chromium are given in Table S1 and Table S2.

TABLE S1. Elastic-properties of single crystal iron and chromium

| **Elastic Properties** | **Iron(Fe)** | **Chromium(Cr)** |
|---|---|---|
| Elastic modulus(GPa) | 211 | 279 |
| Poison ratio | 0.293 | 0.21 |

TABLE S2. Plastic-properties of single crystal iron and chromium

| **Iron(Fe)** | | **Chromium(Cr)** | |
|---|---|---|---|
| Stress(MPa) | Plastic strain | Stress(MPa) | Plastic strain |
| 217.871 | 0 | 290.406 | 0 |
| 221.1009 | 0.00351 | 355.519 | 0.0048 |
| 224.4688 | 0.00903 | 416.759 | 0.0103 |
| 225.6881 | 0.01 | | |

### B. Finite Element Mesh convergence study

To find the optimum mesh size, we compute the true stress-strain curve with 6 different initial skeleton sizes i.e. $25 \times 25, 50 \times 50, 75 \times 75, 100 \times 100, 125 \times 125$, and $150 \times 150$. For this study, we take PF-0.28 and GAN-0.28 microstructures and observe that the results converge for both when we have an initial skeleton size greater than $75 \times 75$. Hence for higher accuracy and computational efficiency, we choose $100 \times 100$ as our initial skeleton size for all microstructures. The result of the mesh convergence study is shown in Figure S1.

### C. Effect of boundary Condition

To assess the effect of Periodic and Kinamatic (Dirichlet) boundary conditions on the PF and GAN generated microstructure, each microstructure is subjected to a standard compression test. For periodic boundary conditions, the centre of the microstructure is fixed, while the top-bottom and left-right nodes are connected by periodic constraints as explained in the manuscript, and for Kinamatic boundary conditions, the left and bottom edge is fixed and a conservative displacement is applied on the right edge through reference point.

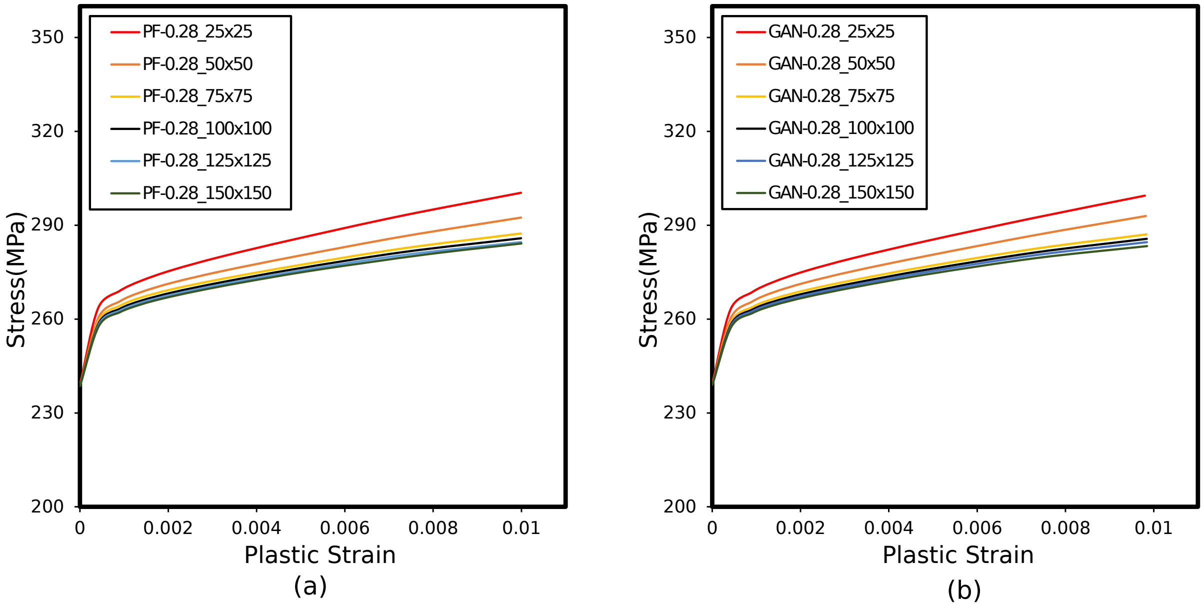


FIG. S1. Mesh convergence study for phase field and GAN generated microstructures in uniform compression for 0.28 composition.

By over-constraining the system, the kinematic boundary condition (KBC) overpredicts mechanical response as KBC restricts deformation freedom at the boundaries (fixed displacements on edges), amplifying stress concentrations near the particles due to the constrained matrix. This constraint forces localized plastic strain to develop around the particles, as the matrix cannot redistribute loads efficiently as compared to periodic boundary conditions (PBC) which enforce displacement continuity between opposing faces and allows cooperative deformation across the matrix to transfer stresses more uniformly around the particles, resulting in an artificially stiffer global response and accelerated hardening as shown in Figure S2.

### D. Error analysis

Figure S3(a) shows the percentage relative error for elasto-plastic response between GAN and PF microstructure. Up to 1 percent plastic strain, the maximum percentage relative error is below 2 percent for all tested compositions. Figure S3(b) shows the mean square error: minimum for 0.28 and below 7.0 for 0.32 composition. The above error analysis shows that for 0.28 and 0.30 compositions, phase-field and GAN results are in excellent agreement

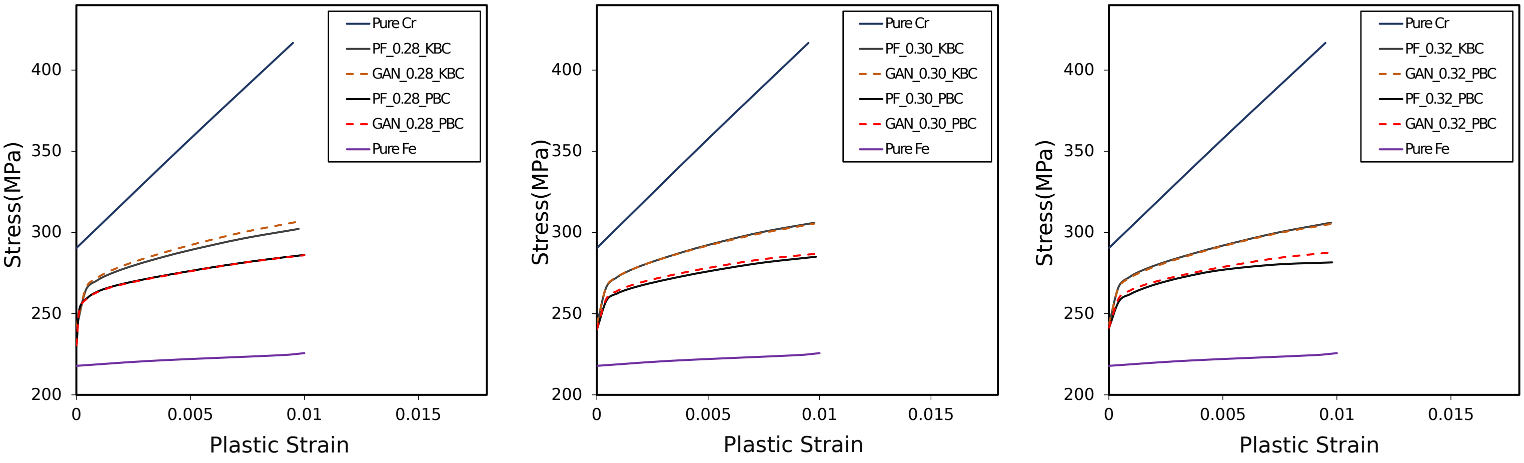


FIG. S2. Effect of Boundary condition for phase field and GAN generated microstructures in uniform compression for 0.28, 0.30, and 0.32 compositions.

with each other. A slightly higher error is observed for 0.32 composition. One can attribute this deviation to the statistical nature of particle distribution, which can vary from one microstructure to another, even for the same volume fraction.

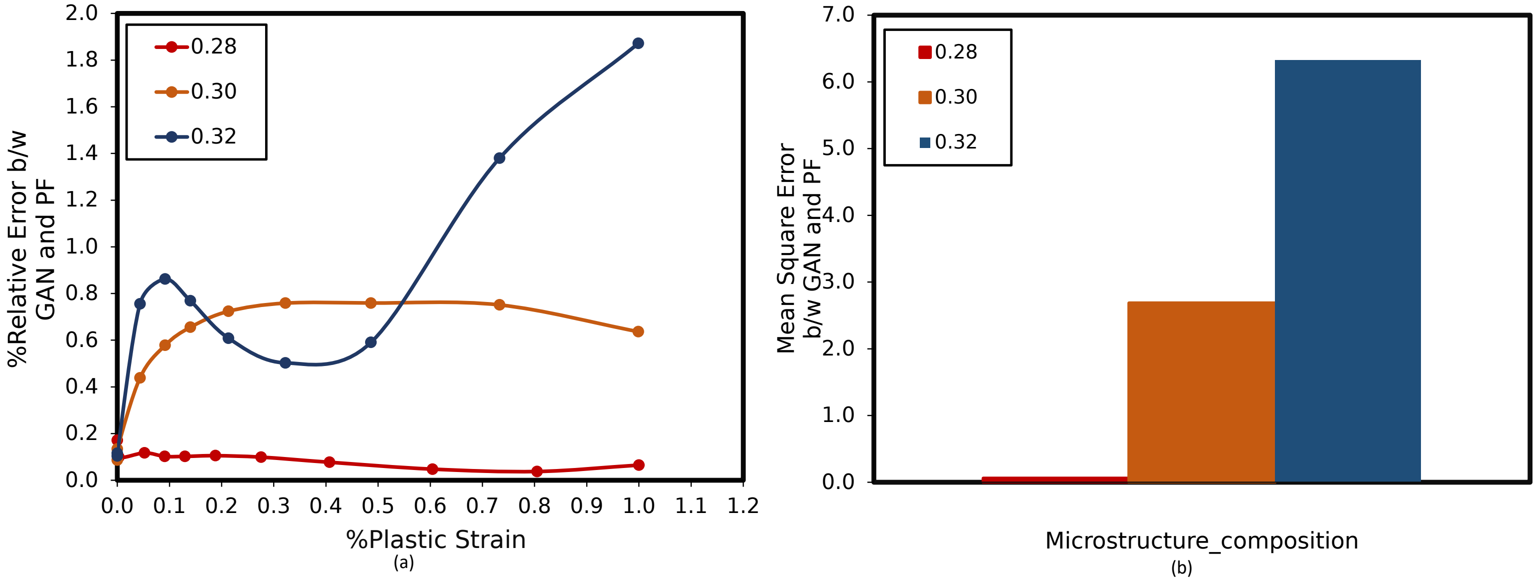


FIG. S3. Error analysis for phase field and GAN generated microstructures (a) Percentage Relative error and (b) Mean square error for 0.28, 0.30, and 0.32 compositions.

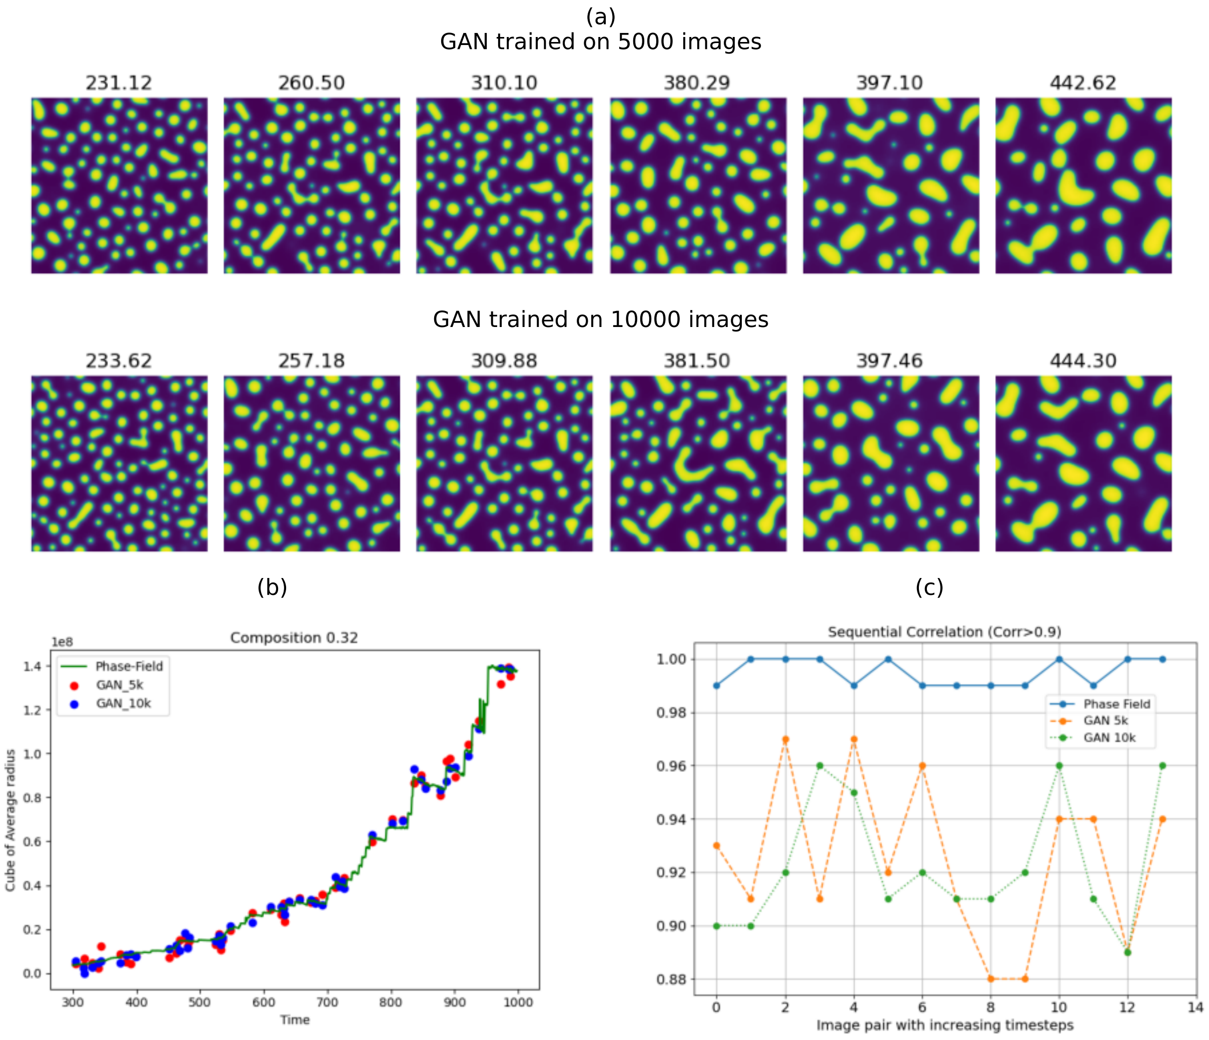


FIG. S4. (a) Synthetic microstructures generated with GAN, using noise as input for initial composition $\phi_A = 0.32$. The top and bottom row shows the output of GAN trained with 5000 and 10000 images, respectively. The average precipitate radius is given in angstrom with every image. (b) Cube of average precipitate radius plotted as a function of time: synthetic microstructures showing the same time dependence as the phase-field microstructures. (c) Synthetic microstructures showing high sequential correlation.

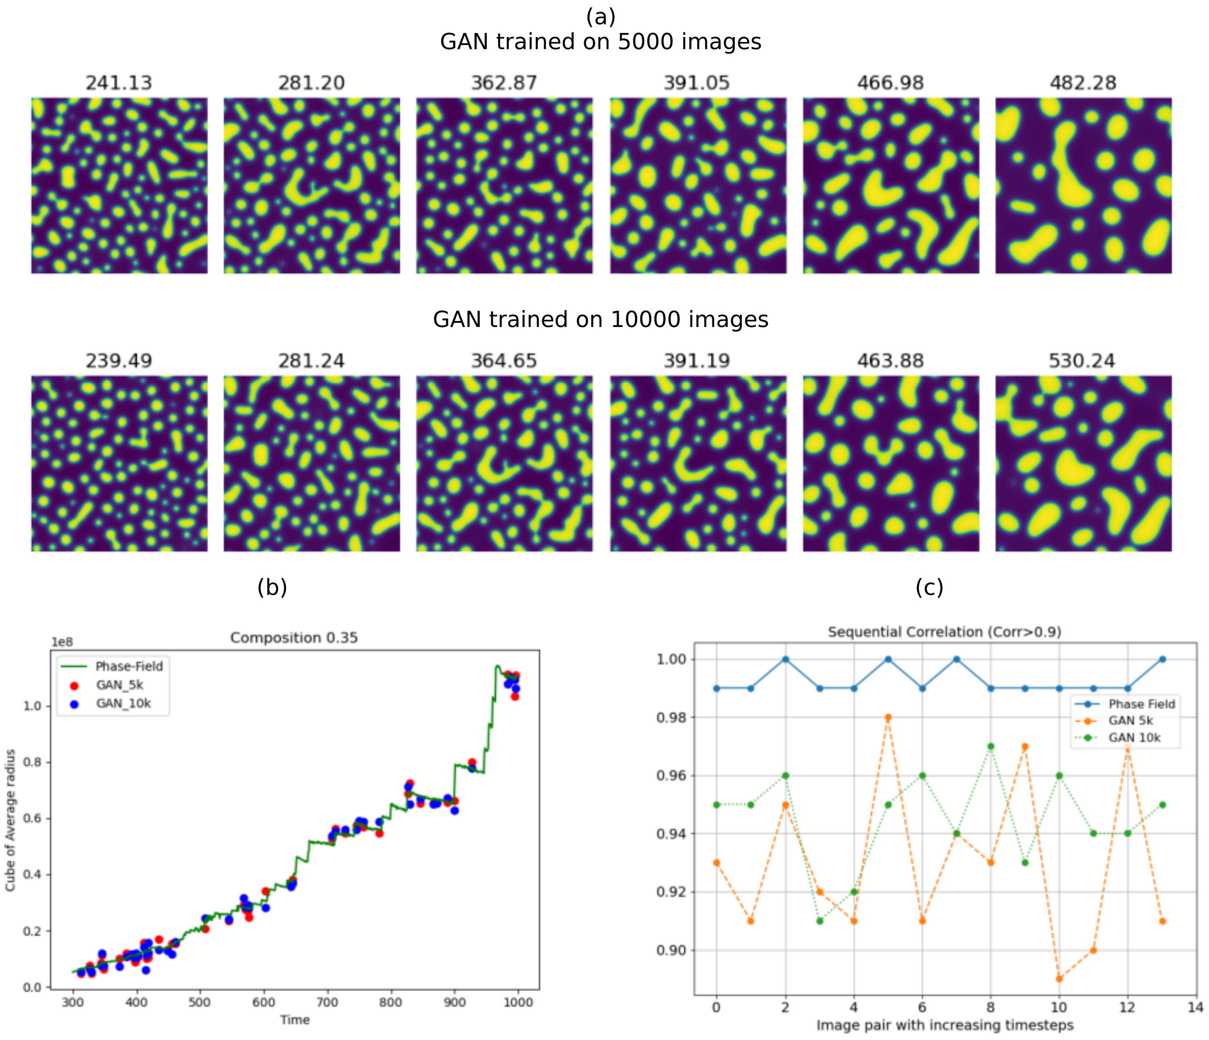


FIG. S5. (a) Synthetic microstructures generated with GAN, using noise as input for initial composition $\phi_A = 0.35$. The top and bottom row shows the output of GAN trained with 5000 and 10000 images, respectively. The average precipitate radius is given in angstrom with every image. (b) Cube of average precipitate radius plotted as a function of time: synthetic microstructures showing the same time dependence as the phase-field microstructures. (c) Synthetic microstructures showing high sequential correlation.

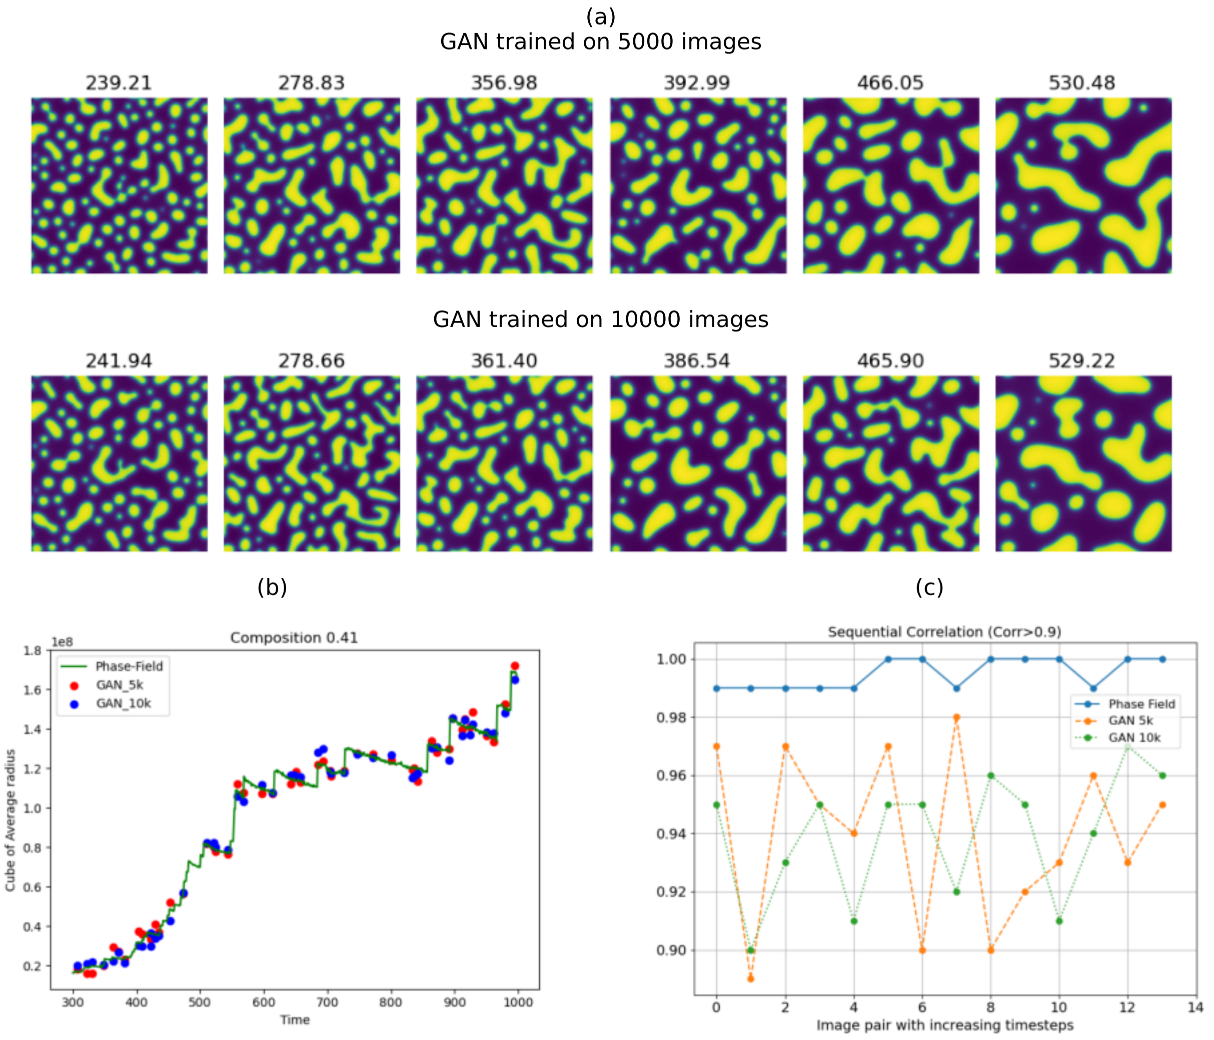


FIG. S6. (a) Synthetic microstructures generated with GAN, using noise as input for initial composition $\phi_A = 0.41$. The top and bottom row shows the output of GAN trained with 5000 and 10000 images, respectively. The average precipitate radius is given in angstrom with every image. (b) Cube of average precipitate radius plotted as a function of time: synthetic microstructures showing the same time dependence as the phase-field microstructures. (c) Synthetic microstructures showing high sequential correlation.

[*] rajdipm@iitk.ac.in

[†] bsomnath@iitk.ac.in

[1] J. W. Cahn and J. E. Hilliard, The Journal of chemical physics **28**, 258 (1958).

[2] J. W. Cahn, Acta metallurgica **9**, 795 (1961).

[3] L. Q. Chen and J. Shen, Computer Physics Communications **108**, 147 (1998).
